# Supplementary material for: A Linter for Isabelle: Implementation and Evaluation
Source: arXiv:2207.10424 source file (2022-07-21)
Supplement: Supplementary file 1 [file 99-appendix.tex]

\begin{table}[!ht]
    \centering
    \begin{tabularx}{\textwidth}{|l|X|}
    \hline
        Bundle Name & Lints \\ \hline
        foundational & Apply-Isar switch, Auto structural composition, Bad-style command, Complex Isar initial method, Complex method, Global attribute changes, Global attribute on unnamed lemma, Implicit rule, Lemma-transforming attribute, Low-level apply chain, Tactic proofs, Unrestricted auto \\ \hline
        default & Apply-Isar switch, Auto structural composition, Axiomatization with where, Bad-style command, Complex Isar initial method, Complex method, Global attribute changes, Global attribute on unnamed lemma, Implicit rule, Lemma-transforming attribute, Low-level apply chain, Short name, SMT oracle, Tactic proofs, Unrestricted auto \\ \hline
        pedantic\_addon & Force failure, Use Isar \\ \hline
        non\_interactive\_addon & Counter-example finder, Diagnostic command, Proof-finder, Unfinished proof \\ \hline
        afp\_mandatory\label{bundle:afp} & Bad-style command, Counter-example finder, Global attribute on unnamed lemma, SMT oracle, Unfinished proof \\ \hline
    \end{tabularx}
    \caption{Lint bundles and their lints}
    \label{tab:bundles}
\end{table}

\begin{table}[!ht]
    \centering
    \begin{tabularx}{\textwidth}{|l|X|}
    \hline
        Option & Description \\ \hline
        \texttt{lint\_bundles} & a comma-separated list of the names of the bundles to be enabled \\ \hline
        \texttt{lints\_enabled} & a comma-separated list of the names
        of the lints to be enabled on top of the enabled bundles\\ \hline
        \texttt{lints\_disabled} & a comma-separated list of the names of the bundles to be disabled \\ \hline
    \end{tabularx}
    \caption{Isabelle Options for the linter}
    \label{tab:options}
\end{table}

\begin{table}[!ht]
    \centering
    \begin{tabularx}{\textwidth}{|l|X|}
    \hline
        Option & Description \\ \hline
        \texttt{linter\_enabled} & indicates whether the linter
        plugin is enabled\\ \hline
        \texttt{lint\_all} & indicates whether the linter
        panel should display all the lints in the theory\\ \hline
        \texttt{lint\_descriptions} & indicates whether the linter
        panel should display the lint descriptions \\ \hline
    \end{tabularx}
    \caption{Isabelle Options for the jEdit linter plugin}
    \label{tab:jedit-options}
\end{table}
